# Supplementary material for: Quantifying intra-regime weather variability for energy applications
Source: arXiv:2408.04302 source file (2024-08-08)
Supplement: Supplementary file 1 [file SI.pdf]

*Geophysical Research Letters*

Supporting Information for

# Quantifying intra-regime weather variability for energy applications

Judith Gerighausen[1], Joshua Dorrington[1, 2], Marisol Osman[1, 3], Christian M. Grams[1, 4]

[1] Institute of Meteorology and Climate Research (IMKTRO), Department Troposphere Research, Karlsruhe Institute of Technology (KIT), Karlsruhe, Germany

[2] now at: Geophysical Institute (GFI), University of Bergen (UiB), Norway

[3] Universidad de Buenos Aires, Facultad de Ciencias Exactas y Naturales, Departamento de Ciencias de la Atmósfera y los Océanos. CONICET – Universidad de Buenos Aires. Centro de Investigaciones del Mar y la Atmósfera (CIMA). CNRS – IRD – CONICET – UBA. Instituto Franco-Argentino para el Estudio del Clima y sus Impactos (IRL 3351 IFAECI)

[4] Federal Office of Meteorology and Climatology, MeteoSwiss, Zurich-Airport, Switzerland

## Contents of this file

Table S1
Figures S1 to S4
Text S1

## Introduction

This Supporting Information provides an overview of the abbreviations used for North Atlantic-European weather regimes (Table S2), and Supporting Figures showing the mean anomalies of 2m temperature (T2m, Figure S1) and 100m wind speed (W100m, Figure S3) during winter (DJF) for all seven North-Atlantic-European weather regimes for ERA5 as well as the respective signal to noise ratios (Figures S2, S4).

Supporting Text S1 explains the Supplementary Dataset with browsable figures, for all regimes, seasons, and countries provided via an open-access data-folder at https://doi.org/10.5281/zenodo.12923703.

| Full name of weather regime | Abbreviation of weather regime |
|---|---|
| Atlantic trough | AT |
| Zonal regime | ZO |
| Scandinavian trough | ScTr |
| Atlantic ridge | AR |
| European blocking | EuBL |
| Scandinavian Blocking | ScBL |
| Greenland Blocking | GL |

**Table S1.** Full name and color code for the seven North-Atlantic European weather regimes and their abbreviation.

**Text S1. Description of the Supplementary Dataset**

A Supplementary Dataset with browsable figures, for all regimes, seasons, and countries is provided at https://doi.org/10.5281/zenodo.12923703 as a zipped archive. As described in the main paper Gerighausen et al. (2024) the analysis is based on ERA5 reanalysis 1979-2021 at 1° grid spacing and 6h temporal resolution aggregated to daily data. Anomalies are computed with respect to a 31-day running mean climatology. The ZIP-File (1.2 GB) contains 4 subfolders and 4 auxiliary files:

**Subfolders**

*./panel/* Panel figures of 5-day running mean surface weather anomalies, fractional standard deviation, and signal-to-noise ratio during all weather regimes together with different contours. The folder is browsable with “PanelPaperPlots.html”. The file naming convention is as follows:
*<variable>/5dr_panel_<type>_<variable>_<season>_<contour>.jpg*

- *<variable>:* SOLD (fraction of maximum possible incoming solar radiation, unitless), T2M (2m temperature in K), TP (total daily precipitation in mm), Wind (100m wind speed in m $s^{-1}$),
- *<type>:* anomaly (mean surface weather anomalies), frac (fractional standard deviation), S2N (signal-to-noise ratio),
- *<season>:* DJF, MAM, JJA, SON,
- *<contour>:* gp (500 hPa geopotential height in gpdm), gpano (500 hPa geopotential height in gpdm), mslp (mean sea level pressure in hPa).

*./violins/* Normed probability density functions (PDF) of country-aggregated surface weather anomaly during each regime and

season displayed as violin plots. The figures are browsable with “PaperPlots.html”. The file naming convention is as follows:

*<country>/<variable>/Violins_<country>_<variable>_<season>. gif*

| | |
|---|---|
| *<country>:* | Austria, Baltics (Lithuania, Latvia, Estonia), Benelux (Belgium, Luxembourg, Netherlands), Bulgaria, Croatia, Cyprus, Czechia, Denmark, Finland, France, Germany, Greece, Hungary, Iceland, Ireland, Italy, Norway, Poland, Portugal, Romania, Slovakia, Slovenia, Spain, Sweden, Switzerland, United Kingdom, |
| *<variable>:* | SOLD, T2M, TP, Wind, (as for “panel”), |
| *<season>:* | DJF, MAM, JJA, SON. |

*./lagged_plots/*

Figures of temporal evolution of the weather regime index IWR in a 20-day window centered on the date of occurrence of a surface weather anomaly for dates in upper and lower terciles of country-aggregated surface weather anomalies during each regime and season. The figures are browsable with “PaperPlots.html”. The file naming convention is as follows:

*<country>/<variable>/<tercile>_lagged_IWRs_<country>_<variable>_<wr>_<season>. gif*

| | |
|---|---|
| *<country>:* | as for violins, |
| *<variable>:* | SOLD, T2M, TP, Wind, (as for “panel”), |
| *<tercile>* | neg (lower tercile of PDF shown in violins), pos (upper tercile of PDF shown in violins), |
| *<wr>* | AT, ZO, ScTr, AR, EuBL, ScBL, GL (weather regime abbreviation as in Table S1), |
| *<season>:* | DJF, MAM, JJA, SON. |

*./extremes/*

Panel figures of mean surface weather anomaly (shading) and 500 hPa geopotential height at (contours in gpdm) during the lower (left) and upper (right) tercile of country-

aggregated surface weather anomalies, and average conditions (middle) during each regime and season. The figures are browsable with “PaperPlots.html”. The file naming convention is as follows:

*<country>/<variable>/*
*Extremes_<country>_<variable>_<wr>_<season>. jpg*

| | |
|---|---|
| *<country>:* | as for violins, |
| *<variable>:* | SOLD, T2M, TP, Wind, (as for “panel”), |
| *<wr>* | AT, ZO, ScTr, AR, EuBL, ScBL, GL (weather regime abbreviation as in Table S1), |
| *<season>:* | DJF, MAM, JJA, SON. |

**Auxiliary files:**

| | |
|---|---|
| *./readme.md* | Description of the contents |
| *./PanelPaperPlots.html* | Navigation panel for browsing plots in folder “panel” of surface weather anomalies of 2m temperature, 100m wind speed, total precipitation, insolation, respective fractional standard deviation, and signal-to-noise ratio during all regimes and seasons. |
| *./PaperPlots.html* | Navigation panel for browsing plots in folders “violins”, “lagged_plots”, “extremes” of country-aggregated surface weather anomalies of 2m temperature, 100m wind speed, total precipitation, insolation for all regimes, seasons, and countries. |
| *./flotplot-scan-min.js* | Javascript functionality for navigation panels. Christopher Polster is acknowledged for providing the Flottplot package at https://chpolste.github.io/flottplot. |

Once downloaded and unpacked in a main folder, the .html navigation panels can be used in any browser to navigate through the plots.

**PanelPaperPlots.html** allows to browse through the anomalies, signal-to-noise ratio (S2N) and fractional standard deviation (FSTD) in all 3-month seasons (winter: December-January-February (DJF), spring: March-April-May (MAM), summer: June-July-August (JJA), autumn: September-October-November (SON)) with the overlay of different isolines (mean sea level pressure with contours every 4 hPa, geopotential height with contours every 10 gpdm and geopotential height anomalies with contours every 4 gpdm). Surface weather anomalies are computed for: 2m temperature in K (T2m), 100m wind speed in m $s^{-1}$ (W100m), total daily precipitation in mm (TP), and

fraction of insolation [0-1] (SOLD). SOLD is defined as the ratio between daily sums of the net solar radiation and the net solar radiation for clear skies at the surface (see Grams et al. 2017).

**PaperPlots.html** allows to browse through country-aggregated surface weather anomalies for countries in the European Economic Area and the European Free Trade Association (stand of 2024). The reader can select the variable, regime, season, and country of interest. Smaller countries are combined (Baltics, Benelux). Countries are masked using the Python package “regionmask” applied to the 1°x1° ERA5 data (https://github.com/regionmask/regionmask, retrieved at 31 July 2024). Displayed are:

1. normed probability density functions (displayed as violin plots) of country-aggregated surface weather anomalies together for all regimes, stratified according to season and country,
2. the temporal evolution of the weather regime index IWR in a 20-day window centered on the date in the upper and lower tercile of a country-aggregated surface weather anomaly stratified according to each regime, season, and country. Significant differences (Kolmogorov-Smirnov test of 1%) between the tercile of interest (solid line) and remaining dates (dashed lines) are marked in bold,
3. maps of mean surface weather anomalies (shading) and 500 hPa geopotential height (contours in gpdm) for dates in the lower and upper tercile of country-aggregated surface weather anomalies, and average conditions stratified according to each regime, season, and country.

The collection of figures complements and can be interpreted along the discussion of selected variables, regimes, seasons, and countries in the the main text of Gerighausen et al. (2024). Please note the changing range of values when comparing plots for different variables, regimes, seasons, or countries.

**References:**

Grams, C., Beerli, R., Pfenninger, S. et al., 2017: Balancing Europe’s wind-power output through spatial deployment informed by weather regimes. *Nature Clim Change* **7**, 557–562, doi:10.1038/nclimate3338, free repository version.

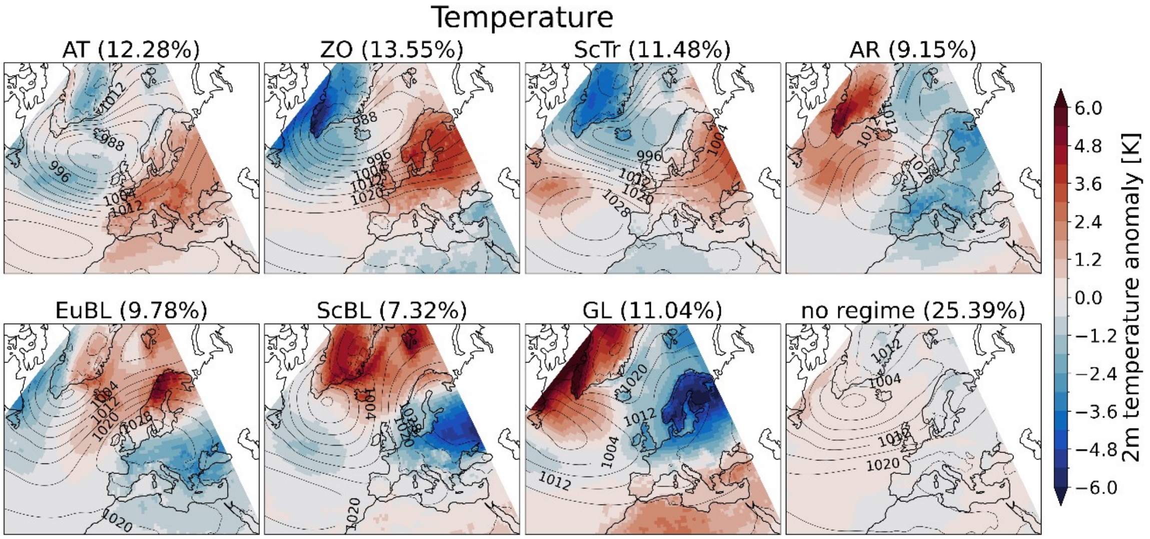


**Figure S1.** Wintertime (DJF) 2m temperature anomalies (shading in K) and mean sea level pressure (contours every 4 hPa) during the seven weather regimes and no regime based on ERA5 reanalysis 1979-2021 at 1° grid spacing. Numbers in brackets above each panel indicate the seasonal occurrence frequency of each regime.

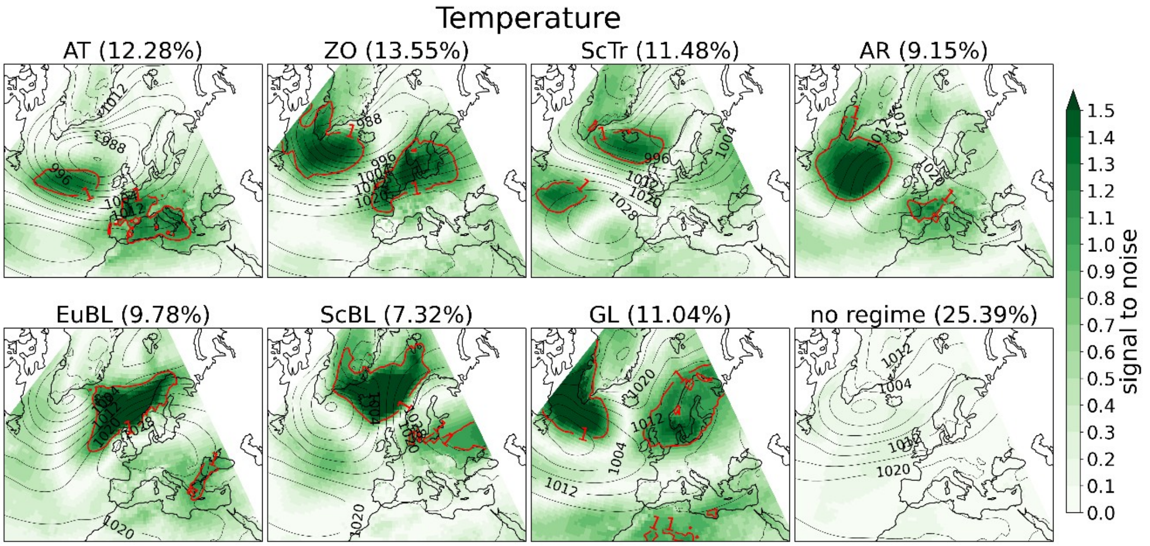


**Figure S2.** Signal to noise ration of wintertime (DJF) 2m temperature anomalies (shading) and mean sea level pressure (contours every 4hPa) during the seven weather regimes and no regime. Numbers in brackets above each panel indicate the seasonal occurrence frequency of each regime.

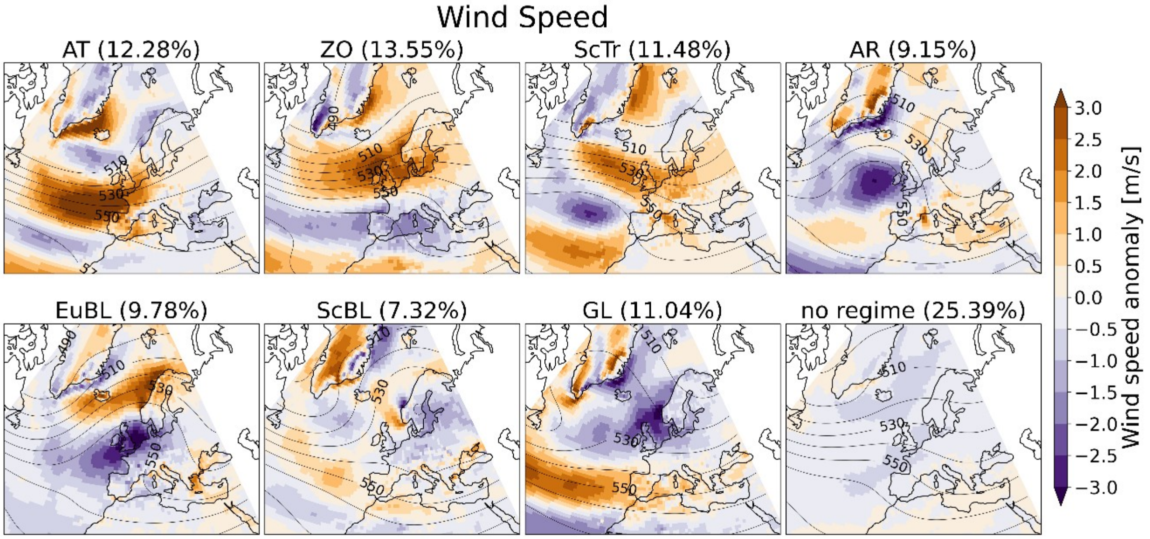


**Figure S3.** Wintertime (DJF) 100m wind speed anomalies (shading in m s$^{-1}$) and geopotential height (contours every 10 gpdm) during the seven weather regimes and no regime based on ERA5 reanalysis 1979-2021 at 1° grid spacing. Numbers in brackets above each panel indicate the seasonal occurrence frequency of each regime.

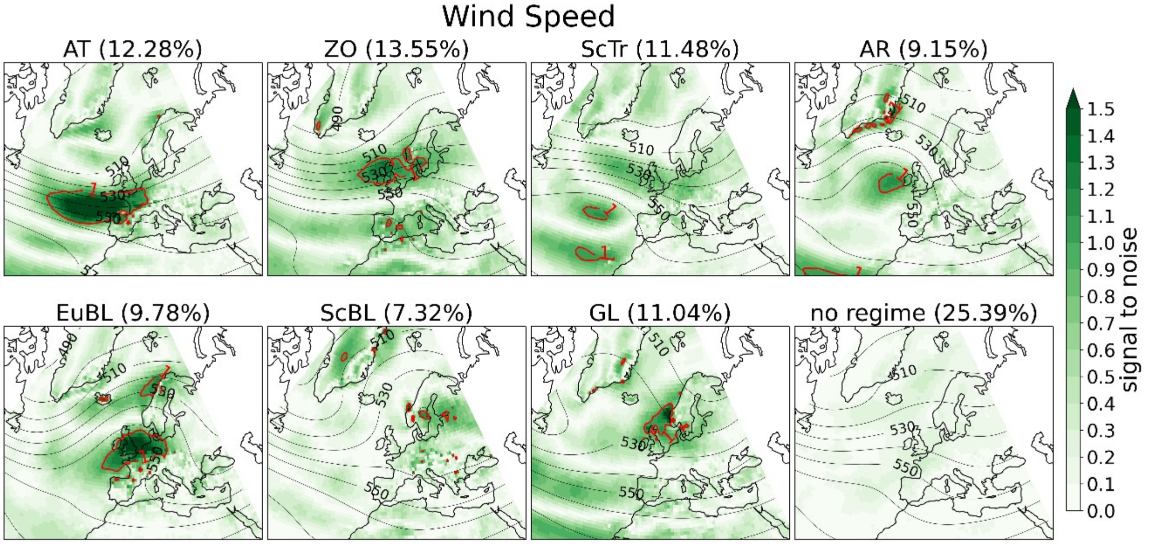


**Figure S4.** Signal to noise ration of wintertime (DJF) 100m wind speed anomalies (shading) and geopotential height (contours every 10 gpdm) during the seven weather regimes and no regime. Numbers in brackets above each panel indicate the seasonal occurrence frequency of each regime.
